# Supplementary material for: Geometric Fabrics: Generalizing Classical Mechanics to Capture the Physics of Behavior
Source: arXiv:2109.10443 source file (2022-01-18)
Supplement: Supplementary file 1 [file appendix_experiments.tex]

%\fullversiononly

\section{Extended Details on Experiments}

\begin{table}[!htb]
	\caption{End-effector target error (ETE) and end-effector wall distance (EWD) as a function of policy class (GF or RMP) and target wall distance (TWD).}
	\label{table:targets_wall}
	\begin{center}
	    \vspace{-4mm}
		\begin{tabular}{| p{1cm} | c | c | c | c |}
		    \hline 
			& ETE (m) & ETE (m) & EWD (m)  & EWD (m)\\
			\hline 
			TWD (m)
			& GF & RMP & GF & RMP\\
			\hline 
			0.3 & 3.041e-5 & 8.09e-05 & 3.0e-1 & 3.001e-1 \\
			\hline 
			0.275 & 2.455e-5 & 7.89e-05 & 2.75e-1 & 2.751e-1 \\
			\hline 
			0.25 & 1.919e-5 & 7.714e-05 & 2.5e-1 & 2.501e-1 \\
			\hline 
			0.225 & 1.432e-5 & 7.568e-05 & 2.25e-1 & 2.251e-1 \\
			\hline 
            0.2 & 1.151e-5 & 7.455e-05 & 2.0e-1 & 2.001e-1 \\
			\hline 
			0.175 & 1.549e-5 & 7.389e-05 & 1.75e-1 & 1.751e-1 \\
			\hline 
			0.15 & 2.88e-5 & 7.564e-05 & 1.5e-1 & 1.501e-1 \\
			\hline 
			0.125 & 5.834e-5 & 1.152e-4 & 1.251e-1 & 1.251e-1\\
			\hline 
			0.1 & 1.564e-4 & 8.482e-4 & 1.002e-1 & 1.009e-1 \\
			\hline 
			0.075 & 1.733e-3 & 8.84e-3 & 7.673e-2 & 8.38e-2 \\
			\hline 
			0.05 & 1.939e-2 & 1.677e-2 & 6.939e-2 & 6.672e-2 \\
			\hline 
			0.025 & 4.315e-2 & 4.351e-2 & 6.816e-2 & 6.846e-2 \\
			\hline 
			0.0 & 6.761e-2 & 9.625e-2 & 6.761e-2 & 9.62e-2 \\
			\hline 
			-0.025 & 9.225e-2 & 1.21e-1 & 6.725e-2 & 9.602e-2 \\
		    \hline 
			-0.05 & 1.17e-1 & 1.459e-1 & 6.698e-2 & 9.595e-2 \\
			\hline 
			-0.075 & 1.418e-1 & 1.715e-1 & 6.683e-2 & 9.651e-2 \\
			\hline 
			-0.1 & 1.668e-1 & 1.957e-1 & 6.681e-2 & 9.571e-2 \\
			\hline 
			-0.125 & 1.919e-1 & 2.214e-1 & 6.691e-2 & 9.644e-2 \\
			\hline 
			-0.15 & 2.171e-1 & 2.457e-1 & 6.709e-2 & 9.581e-2 \\
			\hline 
			-0.175 & 2.422e-1 & 2.714e-1 & 6.724e-2 & 9.647e-2 \\
			\hline 
			-0.2 & 2.673e-1 & 2.957e-1 & 6.732e-2 & 9.578e-2 \\
			\hline 
			-0.225 & 2.924e-1 & 3.213e-1 & 6.735e-2 & 9.638e-2 \\
			\hline 
			-0.25 & 3.173e-1 & 3.455e-1 & 6.737e-2 & 9.564e-2 \\
			\hline 
			-0.275 & 3.424e-1 & 3.712e-1 & 6.737e-2 & 9.636e-2 \\
			\hline 
			-0.3 & 3.674e-1 & 3.961e-1 & 6.738e-2 & 9.632e-2 \\
			\hline
		\end{tabular}
	\end{center}
	\vspace{-4mm}
\end{table}

%\fi
